# Supplementary material for: Dependence of the glass transition and jamming densities on spatial dimension
Source: arXiv:2204.02936 ancillary file (2022-04-06)
Supplement: Supplementary file 1 [file SM_HighD_densities.pdf]

# Dependence of the glass transition and jamming densities on spatial dimension (Supplemental Material)

Monoj Adhikari,[1] Smarajit Karmakar,[2] and Srikanth Sastry[1,*]

[1] *Theoretical Science Unit, Jawaharlal Nehru Centre for Advanced Scientific Research, Jakkur Campus, 560064 Bengaluru, India*
[2] *TIFR Center for Interdisciplinary Science, TIFR, RR District, Hyderabad, 500075, Telangana, India,*

## S1. HOW TO CHOOSE CUTOFF "a"

The parameter "$a$" in the overlap function defined in the main text, is a cut-off chosen to remove any possible decorrelation that might come from the vibrational motions of particles within the cage formed by their respective neighbours [1]. We choose the parameter $a$ in such a way that $a^2$ is close to the plateau value of the mean squared displacement (MSD). The choice of $a$ is further refined by considering the behaviour of $\chi_4$ (defined below), to identify the value of $a$ for which the peak value of $\chi_4$ is maximum. Fig. S1 illustrates the choice for three dimensions (3d at $\phi = 0.8556$), and the $a$ value for other dimensions is chosen by a similar procedure. We choose the parameter values $a = 0.48, 0.50, 0.55, 0.60, 0.75$ ,and 0.80 for 3d, 4d, 5d, 6d, 7d, and 8d, respectively.

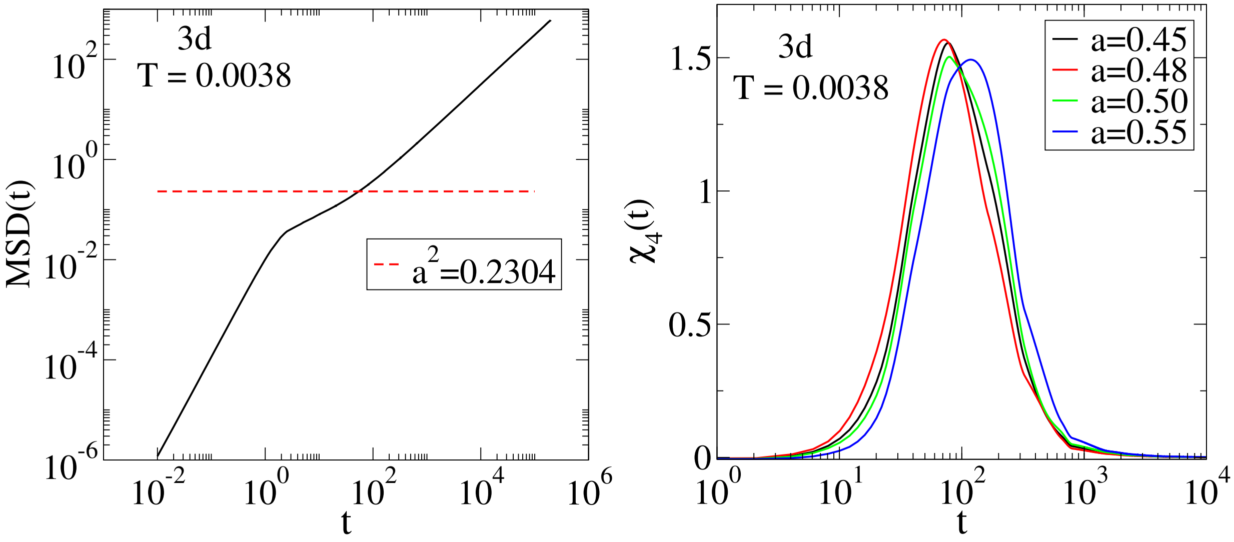


FIG. S1. Choice of the cut-off parameter $a$ for calculating the overlap function, illustrated for 3d, with $T = 0.0038$ as a representative temperature. Left: We show the mean squared displacement (MSD) as a function of time. The horizontal red line corresponds to $a^2 = 0.2304$. Right: $\chi_4(t)$ is shown as a function of time for different $a$ values. The choice $a = 0.48$ leads to the maximum peak value of $\chi_4$.

Dynamical susceptibility, $\chi_4$, which measures the fluctuations in the overlap function $q(t)$, is defined by:

$$\langle \chi_4(t) \rangle = N_B \left[ \langle q(t)^2 \rangle - \langle q(t) \rangle^2 \right] \tag{S1}$$

where $N_B$ is the number of B type particle and $q(t)$ is the overlap function defined in the main text. The average is over initial configurations and the independent samples.

* Corresponding author: sastry@jncasr.ac.in

## S2. SUB-ARRHENIUS TO SUPER-ARRHENIUS BEHAVIOUR AS A FUNCTION OF DENSITY

In order to locate the cross-over density between sub-Arrhenius to super-Arrhenius temperature dependence, we first consider a subset of densities in the vicinity of that density in each dimension (the full set of data are shown in Fig. 1 in the main text). For such subsets of densities, we fit the $\tau_\alpha$ at high temperatures to an Arrhenius form

$$\tau_\alpha = \tau_0 \exp\left(\frac{A}{k_B T}\right). \tag{S2}$$

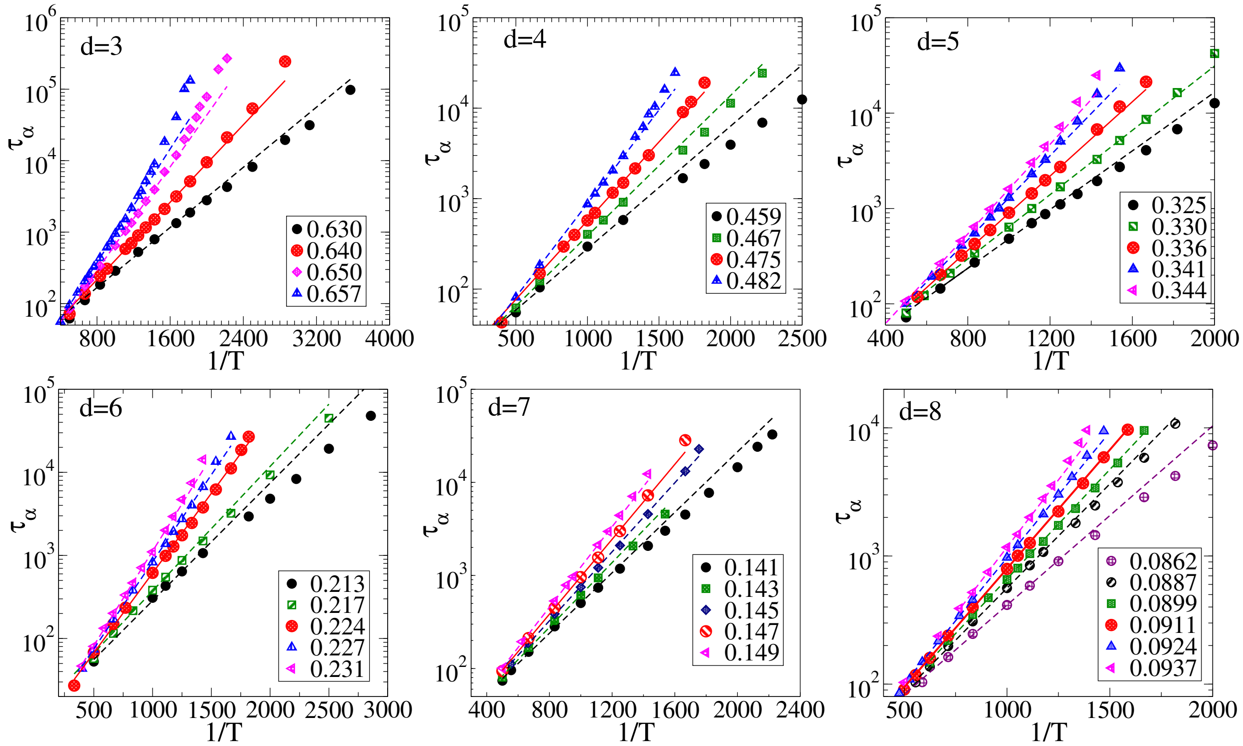


FIG. S2. Relaxation time is plotted as a function of inverse temperature and fitted with the Arrhenius form at high temperatures. The points correspond to simulation data. Lines are fits to Arrhenius form.

In Fig. S2, we show the Arrhenius fits in each dimension, which demonstrates that the change from sub-Arrhenius to super-Arrhenius temperature dependence of the relaxation times occurs within the range of densities shown. We use these density ranges as an initial bounding range of $\phi_0$ in the scaling analysis of dynamics.

## S3. SCALING ANALYSIS OF DYNAMICS

### A. Berthier-Witten (BW) scaling

As described in the main text, we obtain the crossover density, $\phi_0$ in $3-8$ spatial dimensions, using the scaling form proposed by Berthier and Witten (BW) [2] (in addition to the newly proposed form described below):

$$\sqrt{T}\tau_\alpha(\phi,T) \sim \exp\left[\left(\frac{A}{|\phi_0-\phi|^\delta}\right) F_\pm\left(\frac{|\phi_0-\phi|^{\frac{2}{\mu}}}{T}\right)\right]. \tag{S3}$$

In Fig. S3, we show the scaling plots of relaxation times (BW scaling) for $3-8$ spatial dimensions. In performing the data collapse, we consider the densities within the bounding ranges identified above. We further impose the condition $\mu\delta/2 = 1$ so that the scaling form in Eq. S3 leads to an Arrhenius form at $\phi_0$. We compute a quantification of the error, $\chi^2_\tau$, as detailed below in Sec. S5 for a range of $\phi_0$ and $\delta$ values, and identify the $\phi_0$ and $\delta$ values that minimize $\chi^2_\tau$. The values of $\chi^2_\tau$ *vs.* $\phi_0$ and $\delta$ are not smooth, for reasons we describe below. Thus, after we identify the $\phi_0$ and $\delta$ values that minimize $\chi^2_\tau$, we consider small variations around such values in order to improve the quality of the data collapse of $\tau_\alpha$ into two branches across $\phi_0$. The best estimates of $\phi_0$ are shown in the legends in Fig. S3, and error bars, obtained by considering an increase in $\chi^2_\tau$ by 20% of the lowest value, are shown in Table S1.

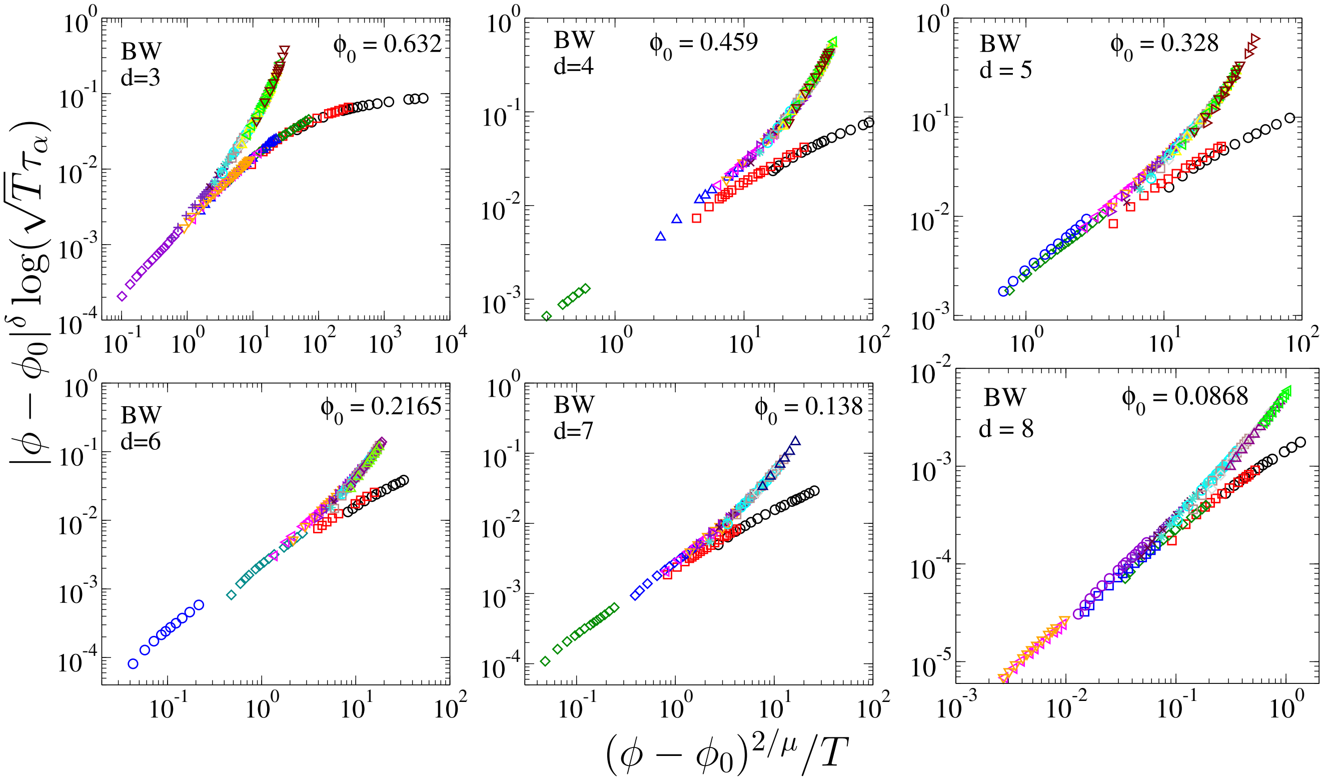


FIG. S3. Data collapse of relaxation times using the Berthier-Witten scaling function. The estimated $\phi_0$ values are shown in the legends.

### B. New effective diameter definition and scaling function

In our analysis in the present work, we obtain an expression for the density-temperature dependent effective density using the effective diameter proposed by Barker and Henderson in [3]. We do not consider other improvements to the Barker-Henderson expression commonly used in liquid-state theory, as we wish to analyse the dynamical data with a

minimal set of parameters, which nevertheless will be accurate in capturing low temperature behavior. Following [3], we have

$$\sigma_{eff} = \int [1 - \exp(-\beta u(r))]\, dr \tag{S4}$$

where $\beta = 1/k_B T$, and $u(r)$ is the pairwise interaction potential. For the harmonic pair potential we consider, we have

$$\sigma_{eff} = \int_0^{\sigma} \left[1 - \exp\left(-\beta\left(1 - \frac{r}{\sigma}\right)^2\right)\right] dr. \tag{S5}$$

Integrating the above equation,

$$\sigma_{eff} = \sigma\left[1 - \frac{1}{2}\sqrt{\frac{\pi}{\beta}}\, erf(\sqrt{\beta})\right] \tag{S6}$$

Since we are interested in low temperatures, we use the approximation $erf(\sqrt{\beta}) \approx 1$, and verify that it leads to negligible errors compared to the expression in Eq. S6 for the temperature range relevant to our work.

Thus, the effective diameter used in this work is

$$\sigma_{eff} = \sigma\left[1 - \frac{1}{2}\sqrt{\frac{\pi}{\beta}}\right] \tag{S7}$$

employing which, we have

$$\sigma_{eff}^d = \sigma^d\left[1 - \frac{d\sqrt{\pi}}{2}\sqrt{T} + \frac{d(d-1)\pi}{8}T - \mathcal{O}\left(T^{3/2}\right)\right]. \tag{S8}$$

In order to express the effective volume fraction $\phi_{eff}$ ($\propto \sigma_{eff}^d$ in dimension $d$) with a small number of parameters, we approximate it as

$$\phi_{eff} \sim \phi\left(1 - a\,\sqrt{T} + b\,T^{\beta}\right). \tag{S9}$$

where $a = \frac{d\sqrt{\pi}}{2}$ is kept fixed according to Eq. S8 in the following, and we allow $b$ and $\beta$ to be fitting parameters, with $\beta > 0.5$. This introduces one additional parameter as compared to BW scaling, but as described below, we employ equation of state data to fix the parameters $b$ and $\beta$ and thus scale dynamical data employing only $\phi_0$ and $\delta$ as parameters to be determined.

Assuming that relaxation times for the hard sphere fluid follow

$$\sqrt{T}\tau_\alpha^{hs} \sim \exp\left[\frac{A}{(\phi_0 - \phi)^\delta}\right], \tag{S10}$$

and employing Eq. S9 for the effective diameter, we have

$$\sqrt{T}\tau_\alpha(\phi, T) \sim \exp\left[\frac{A}{(\phi_0 - \phi)^\delta\left(1 - \frac{\phi(a\sqrt{T} - bT^\beta)}{\phi_0 - \phi}\right)^\delta}\right] \tag{S11}$$

based on which, we write a scaling form

$$\sqrt{T}\tau_\alpha(\phi, T) \sim \exp\left[\left(\frac{A}{|\phi_0 - \phi|^\delta}\right) F_\pm\left(\frac{|\frac{\phi_0}{\phi} - 1|}{a\sqrt{T} - bT^\beta}\right)\right] \tag{S12}$$

where $F_\pm(x)$ refer to the scaling functions for the super-Arrhenius and the sub-Arrhenius branches.

The estimation of parameters $b$ and $\beta$ from equation of state data is described below in Sec. S4. Following such estimation, we consider data collapse of $\tau_\alpha$ according to Eq. S12. To this end, we compute the error $\chi_\tau^2$ as described in Sec. S5 for a range of choices of $\phi_0$ and $\delta$, with $\phi_0$ within the bounding range described earlier. As discussed in Sec. S5, we find a range of combinations of $\phi_0$ and $\delta$ values for which $\chi_\tau^2$ is comparable, similar to observations in [4]. Hence, we employ the constraint that the scaling form in Eq. S12 must reduce to the Arrhenius form at $\phi_0$, and fix the value of $\delta = 2$. With such a choice, $\phi_0$ remains the only parameter to be estimated, which we estimate as the value that minimizes $\chi_\tau^2$. The best estimates of $\phi_0$ are shown in the legends in Fig. 2 of the main text, and error bars, obtained by considering an increase in $\chi_\tau^2$ by 20% of the lowest value, are shown in Table S1 and Table 1 of the main text.

### C. Comparison of $\phi_0$ from different procedures

Here we tabulate the $\phi_0$ estimates obtained from the different scaling procedures we employ: (i) the BW scaling (shown above) (BW), and (ii) the new scaling procedure where $b$ and $\beta$ is obtained from the equation of state data collapse, $\delta$ set to 2 and $\phi_0$ estimated from the data collapse of relaxation times (shown in the main text) (AKS). Table S1 demonstrates that the $\phi_0$ values obtained are consistent with each other. We also include the theoretical Kauzmann density values calculated in [5] (MZ).

| Dimension | BW | AKS | MZ [5] |
|---|---|---|---|
| 3 | $0.632 \pm 0.001$ | $0.644 \pm 0.003$ | 0.624414 |
| 4 | $0.459 \pm 0.001$ | $0.462 \pm 0.004$ | 0.480302 |
| 5 | $0.328 \pm 0.001$ | $0.325 \pm 0.003$ | 0.325298 |
| 6 | $0.214 \pm 0.0005$ | $0.214 \pm 0.002$ | 0.203008 |
| 7 | $0.138 \pm 0.0005$ | $0.140 \pm 0.002$ | 0.126974 |
| 8 | $0.0868 \pm 0.0002$ | $0.0870 \pm 0.001$ | 0.0777626 |

TABLE S1. Densities $\phi_0$ obtained from different scaling procedures, and from theoretical estimates in [5], shown for $3 - 8$ spatial dimensions.

## S4. ESTIMATING PARAMETERS $b$ AND $\beta$ FROM EQUATION OF STATE DATA

We describe here how we estimate $b$ and $\beta$, mentioned earlier in Sec. S3.B. The pressure $P$ is evaluated at each state point, in each dimension, as a function of $\phi$ and T, *i.e.* $P = f(T, \phi)$. For a suitable choice of the effective volume fraction $\phi_{eff}(\phi, T)$, we may expect $P$ to be a unique function of $\phi_{eff}$. Thus, with the chosen form

$$\phi_{eff} = \phi(1 - a\sqrt{T} + bT^\beta) \tag{S13}$$

we require that $Z \equiv P/\rho T$, plotted as a function of $\phi_{eff}$ should exhibit a data collapse for the full set of densities and temperatures in each dimension, and use this to obtain the best fit values of $b$ and $\beta$, keeping the choice of $a$ fixed to values given in Eq. S8. We compute the error of the pressure collapse as follows. The range of $x$ (or $\phi_{eff}$) values is divided into bins of width $\delta x$ (we choose $\delta x = 0.05$), and each bin is indexed by $i$, with $n_i$ data points, from different density, temperature data sets. For each bin, we compute a mean $y$ value $\langle y_i \rangle = \frac{1}{n_i} \sum_{j=1}^{n_i} y_j$. We then define

$$\chi^2 = \frac{1}{tot_{bin}(n_i > 1)} \sum_{i(n_i>1)} \frac{1}{n_i} \sum_{j=1}^{n_i} [y_i(j) - \langle y_i \rangle]^2 \tag{S14}$$

where $tot_{bin}(n_i > 1)$ is the total number of bins with more than one data point. We observe that in each dimension the best estimate of $\beta$ is close to 0.7. Thus, we employ $\beta = 0.7$ for all dimensions, and estimate $b$ values that minimize $\chi^2$, considering integer increments in $b$. The estimated $b$ values are shown in the legends in Fig. 2 of the main text. We note that the best fit $b$ values change between values $-5.0$ and $-7.0$ non-monotonically as the dimension is varied, which point to inadequacies of the data set or form of the effective volume fraction we have considered, which should be investigated further. However, we note that a change in the $b$ values used, between $-7.0$ and $-5.0$ leads to insignificant changes in the $\phi_0$ values we estimate.

## S5. ERROR ANALYSIS FOR THE SCALING OF RELAXATION TIMES

We describe here the estimation of parameters that lead to scaling collapse of the relaxation times into two scaling functions above and below the density $\phi_0$, with explicit reference to the new scaling form shown in Eq. S12 wherein the parameters describing the effective packing fraction $\phi_{eff}$ have been determined through the equation of state. In this case, only the parameters $\phi_0$ and $\delta$ need to be determined. We follow a similar procedure for the case of the Berthier-Witten scaling form in Eq. S3. For each choice of the fitting parameters, we define an error $\chi_\tau^2$ as follows: For each choice of $\phi_0$, the range of densities is divided into a subset with $\phi > \phi_0$ and $\phi < \phi_0$, for each of which we define ${\chi_\tau^{\pm}}^2$, and define $\chi_\tau^2 = {\chi_\tau^+}^2 + {\chi_\tau^-}^2$ where $+$ corresponds to the set $\phi > \phi_0$ and $-$ corresponds to the set with $\phi < \phi_0$. For each subset of data, for each data point, we define an $x$ value and a $y$ value, with $x = \log\left(\frac{|\frac{\phi_0}{\phi}-1|}{a\sqrt{T}-bT^\beta}\right)$ and $y = \log\left[|\phi_0-\phi|^\delta \log\left(\sqrt{T}\tau_\alpha(\phi,T)\right)\right]$. The range of $x$ values is divided into bins of width $\delta x$ (we choose $\delta x = 0.05$), and each bin is indexed by $i$, with $n_i^\pm$ data points for the two subsets. For each bin, and for each subset, we compute a mean $y$ value $\langle y_i^\pm\rangle = \frac{1}{n_i^\pm}\sum_{j=1}^{n_i^\pm} y_j^\pm$ (for bins with $n_i^\pm \neq 0$, $\langle y_i^\pm\rangle = 0$ otherwise). We then define

$$
{\chi_\tau^{\pm}}^2 = \frac{1}{tot_{bin}(n_i > 1)} \sum_{i(n_i^\pm > 1)} \frac{1}{n_i^\pm} \sum_{j=1}^{n_i^\pm} \left[y_i^\pm(j) - \langle y_i^\pm\rangle\right]^2 \tag{S15}
$$

from which the total error $\chi_\tau^2$ is computed, and minimized with respect to the parameters sought to be estimated ($\phi_0$ and $\delta$). We note that the quantity $\chi_\tau^2$ is not a smooth function of the parameters $\phi_0$ and $\delta$, since the number of points $n_i$ in each bin can change discontinuously with a variation of $\phi_0$ and $\delta$. Further, for some choices of $\phi_0$ and $\delta$, low values of $\chi_\tau^2$ can be obtained for relatively poor scaling collapse, arising from the fact that several bins of $x$ values contain a single data set and hence does not contribute to the error. Thus, (only in the case of BW scaling) after we obtain estimates of $\phi_0$ and $\delta$ that minimize $\chi_\tau^2$, we consider small variations around these values that improve upon the scaling collapse. Finally, for the scaling function Eq. S12, we fix the value of $\delta$ to be $\delta = 2$, which we justify below.

### A. Justification of the choice $\delta = 2$

Based on the scaling function Eq. S12 we propose, a natural choice for the value of $\delta$ is 2, which leads to an Arrhenius form at low temperatures at the crossover density $\phi_0$. The value $\delta = 2$ is also what has been argued to be valid in 3 dimensions [6], and close to the value found in [2, 7]. Nevertheless, the value of $\delta$ in higher dimensional hard sphere fluids is not available, and therefore, we consider initially the variation of $\delta$, along with $\phi_0$, in Eq. S12, after fixing $b$ and $\beta$ using equation of state data. We compute the error as described above for a range of choices of $\phi_0$ and $\delta$, which is shown in Fig. S4 for $d = 3$. We note that a range of $\phi_0$ values and corresponding $\delta$ values exhibit comparable errors. In Fig. S5 we show the minimum of $\chi_\tau^2$ for each $\phi_0$ and plot it as a function of $\phi_0$ (left) and equivalently, the corresponding $\delta$ (right). Though the errors are comparable for the range of $\phi_0$ and $\delta$ we consider, minimum errors are obtained for $\delta$ values close to $\delta = 2$. Similar results are also obtained for all other dimensions. On this basis, we conclude that the choice $\delta = 2$ is reasonable, which we fix in subsequent analysis, and estimate $\phi_0$ based on minimizing $\chi_\tau^2$, as shown in Fig. S6.

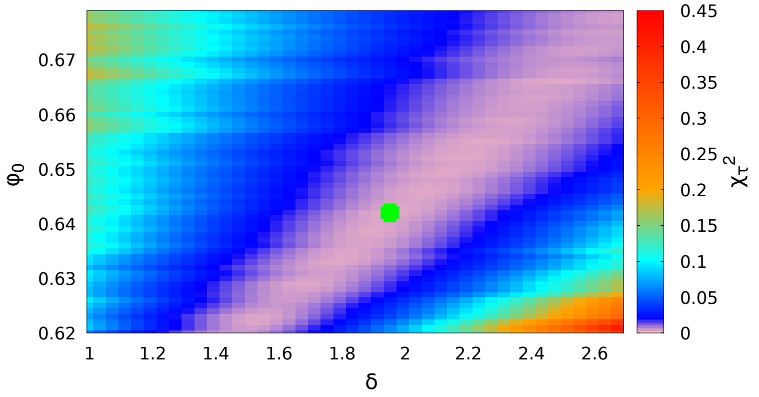


FIG. S4. Heat map of error $\chi^2_\tau$ as a function of $\phi_0$ and $\delta$ for a big range of $\delta$ and $\phi_0$. The green dot indicates the values of $\phi_0$ and $\delta$ for which $\chi^2_\tau$ is minimum.

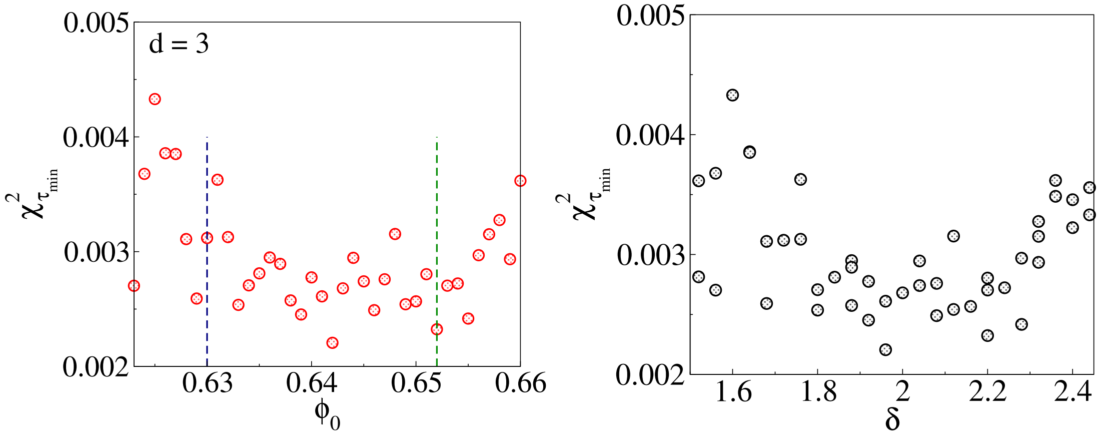


FIG. S5. For each $\phi_0$, we obtain the value of $\delta$ for which $\chi^2_\tau$ is minimum. The minimum $\chi^2_\tau$ so obtained is plotted as a function of $\phi_0$ (left) and alternately, the corresponding $\delta$ (right). The vertical lines indicate the range of $\phi_0$ within which we estimate the best fit value, as described in Sec. S1.

## S6. JAMMING DENSITY OF SOFT SPHERE

We calculate the jamming density for soft sphere system for $3-8$ dimension by following the steps given below:

- We choose the initial positions of the spheres randomly at a low density, such that the energies of the configurations are zero.
- We compress the system by uniformly inflating all the particle diameters.
- After each step of compression (compression step: 0.0001 for $d=3,4$ 0.00005 for $d=5,6$, 0.00001 for $d=7$ and $8\times10^{-5}$ for $d=8$) the potential energy of the system is minimized using the conjugate gradient method.
- We continue this process until the system reaches the energy of the order of $10^{-5}$.
- To locate the jamming density, we slowly (10 times slower than the compression) decompress the system, minimizing the energy at each step of decompression.
- We continue decompression until the energy of the system becomes less than $10^{-16}$. The density at which energy reaches $10^{-16}$ is the estimate used of the jamming density.
- The above procedure is repeated for 1000 independent configurations, to obtain the average jamming density and the corresponding distribution.

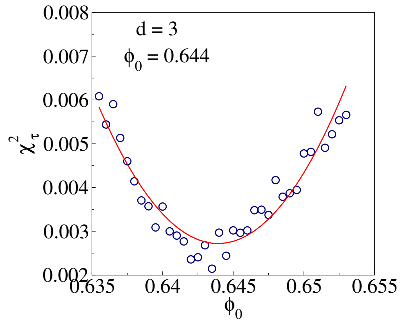


FIG. S6. $\chi^2_\tau$ as a function of $\phi_0$, with $\delta = 2.0$.

In Fig. S7, we show the energy as a function of density for different initial samples during the compression and decompression cycles. The histogram of jamming densities are shown in Fig. S8. A comparison of the jamming densities we obtain and in previous works is shown in Table S2.

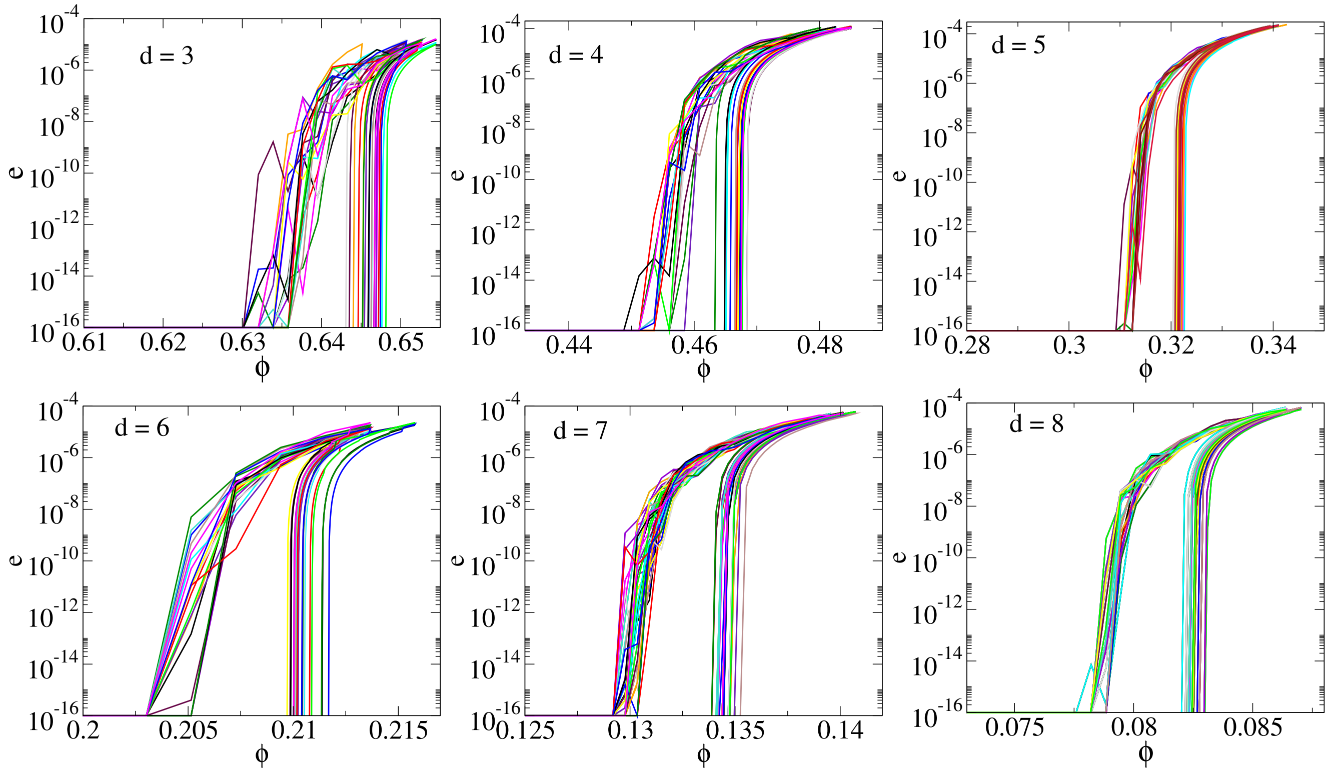


FIG. S7. Energy as a function of density $\phi$ during the compression and decompression cycles. Different lines correspond to different initial conditions (We show here 50 samples).

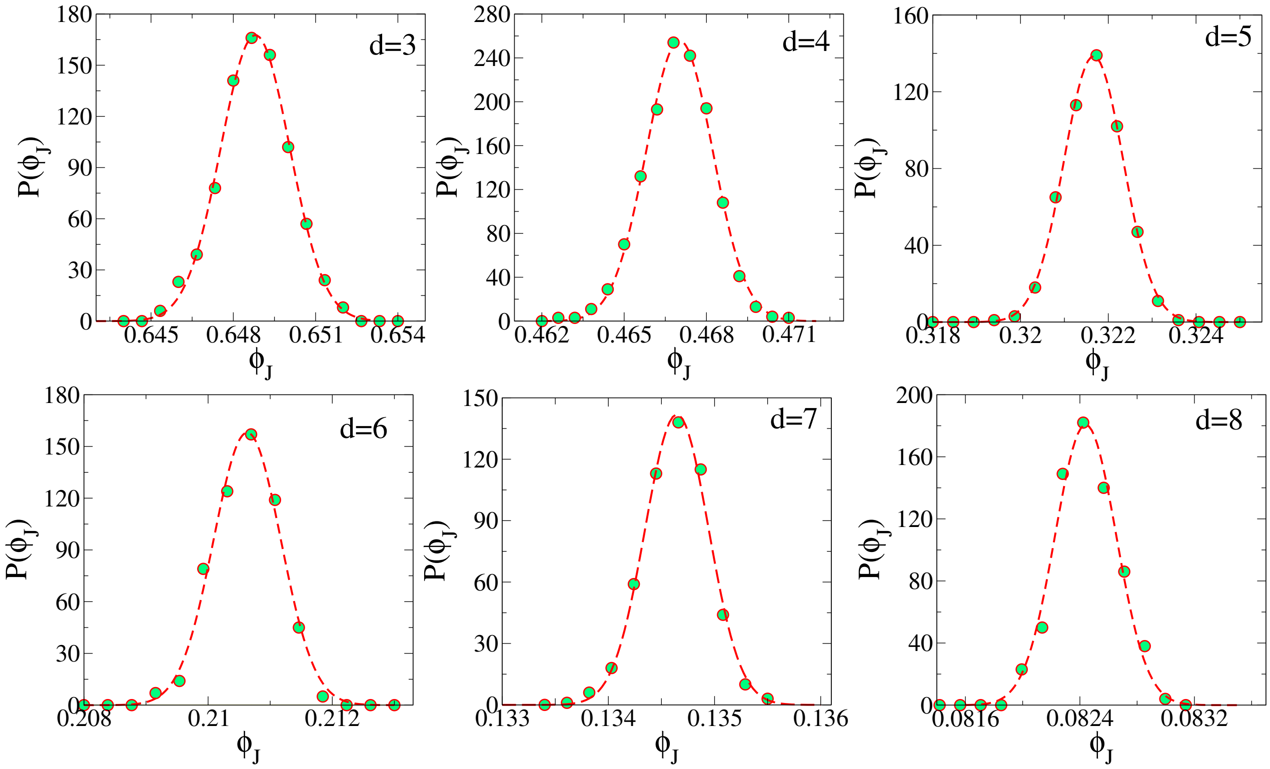


FIG. S8. Histogram of the jamming densities $\phi_J$ obtained from 1000 samples are shown for $3-8$ spatial dimensions.

| Dimension | Our work | Charbonneau *et al.* ($\phi_{th}$) [8] | Morse *et al.* [9] | Charbonneau *et al.* [10] |
|---|---|---|---|---|
| 3 | $0.648 \pm 0.0014$ | 0.651 | 0.6472 | 0.6487 |
| 4 | $0.467 \pm 0.0015$ | 0.467 | 0.4636 | 0.4564 |
| 5 | $0.320 \pm 0.0008$ | 0.319 | 0.3155 | 0.3083 |
| 6 | $0.209 \pm 0.0006$ | 0.209 | 0.2066 | 0.2008 |
| 7 | $0.1345 \pm 0.0004$ | 0.133 | 0.1309 | |
| 8 | $0.0824 \pm 0.0003$ | 0.0821 | 0.0809 | |

TABLE S2. Densities $\phi_J$ computed in the present work, with a comparison with previous works, shown for $3-8$ spatial dimensions. Error bars are obtained as the half width at half maximum of the distributions shown in Fig. S8.

## S7. DENSITY-TEMPERATURE DIAGRAM

We show here the density-temperature diagram, indicating all the temperatures and densities at which simulations are performed, along with the density dependent $T_{VFT}$, and the densities $\phi_0$ for all the spatial dimensions investigated. In all dimensions, except in $d = 5, 8$, the fitted VFT temperatures extrapolate convincingly to zero as $\phi \to \phi_0$. For $d = 5, 8$, the VFT temperatures become very small for slightly higher temperatures, but since at these dimensions, $\phi_J < \phi_0$, even in these cases, $\phi_0$ is a better candidate for the limit density at which $T_{VFT} \to 0$ than $\phi_J$. Relaxation times over a more extended temperature range are required for a better analysis than that presented.

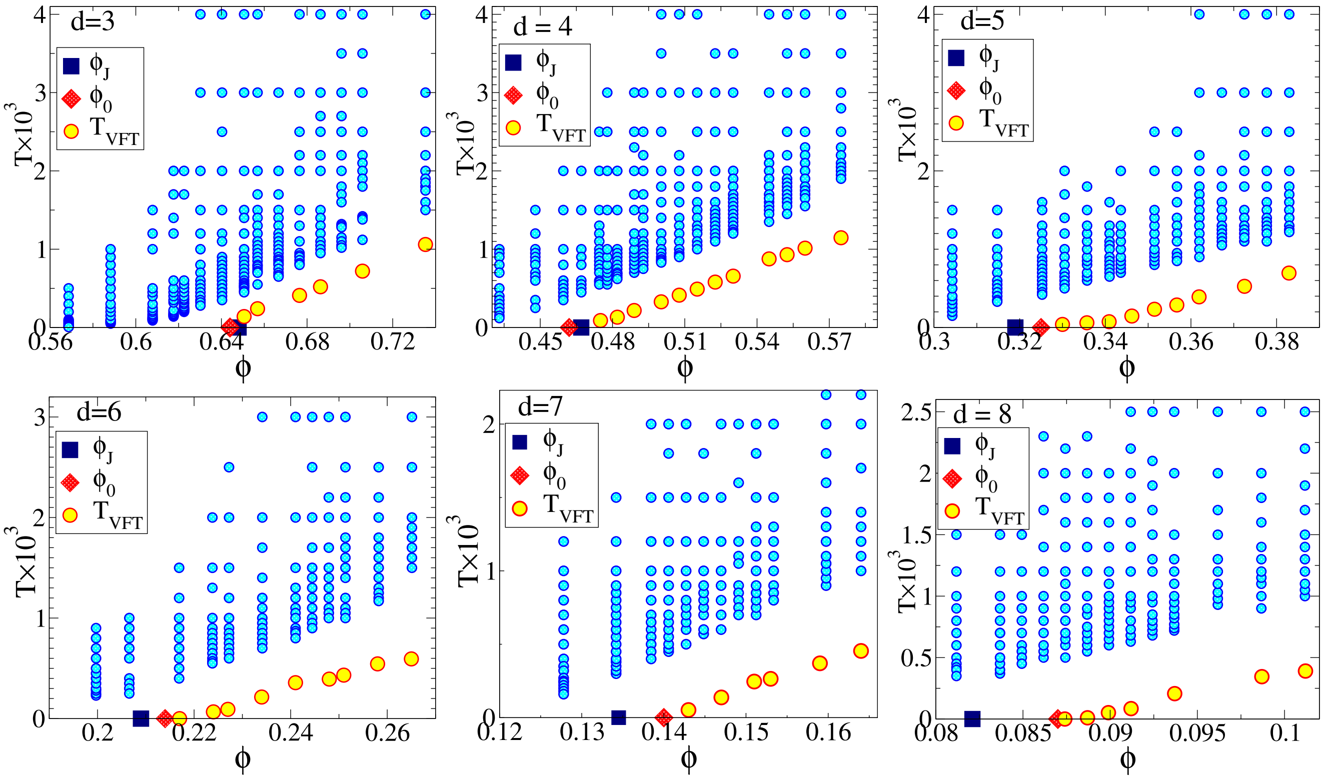


FIG. S9. The jamming and glass transition densities $\phi_J$ (black square) and $\phi_0$ (red diamond) are shown for $d = 3$ to $d = 8$ along with the density dependent glass transition temperatures $T_{VFT}$ (orange circles), and the set of densities and temperatures at which simulations have been performed (blue circles).

## S8. FRACTION OF RATTLERS AS A FUNCTION OF DENSITY

To explore a possible connection between $\phi_0$ and densities other than $\phi_J$, we compute the density at which the fraction of rattler becomes zero. We compute the fraction of rattlers as a function of density in $3-8$ spatial dimensions. First, the system is equilibrated at a temperature at which $\tau_\alpha \sim 10$. Then, the equilibrated liquid is quenched to zero temperature employing the conjugate gradient minimization minimization. We compute the Hessian matrix for such energy minimum configurations and compute the eigenvalues of the Hessian matrix. The Hessian matrix is defined as

$$\mathcal{H}_{ij}^{\alpha\beta} = \frac{\partial^2 U}{\partial r_i^\alpha \partial r_j^\beta}, \tag{S16}$$

where, $i$ and $j$ refer to particle $i$ and $j$. $\alpha$ and $\beta$ correspond to different spatial directions varying from 1 to $d$. $U$ is the total potential energy of the system and $r_i^\alpha$ is the $\alpha^{th}$ component of the position vector of particle $i$. For a system of $N$ particles, the Hessian matrix will be of size $Nd \times Nd$. In $d$ dimensions, there will be at least $d$ eigenvalues which are zero (corresponding to global translations). If there are more than $d$ eigenvalues which are zero, they arise from the presence of rattlers. The fraction of ratters, $f_R$ is the total number of zero eigenvalues (minus $d$) divided by the total number of eigenvalues. In Fig. S10, we show the fraction of rattlers, $f_R$, as a function of density (scaled with jamming density, $\phi_J$) for $3-8$ spatial dimension. The density at which $f_R$ reaches a threshold value of $10^{-5}$ is termed as $\phi_{nr}$. We see that this density neither corresponds to $\phi_J$ nor $\phi_0$. This density turns out to be larger than $\phi_0$ for all dimensions, and thus bears no relation to $\phi_0$.

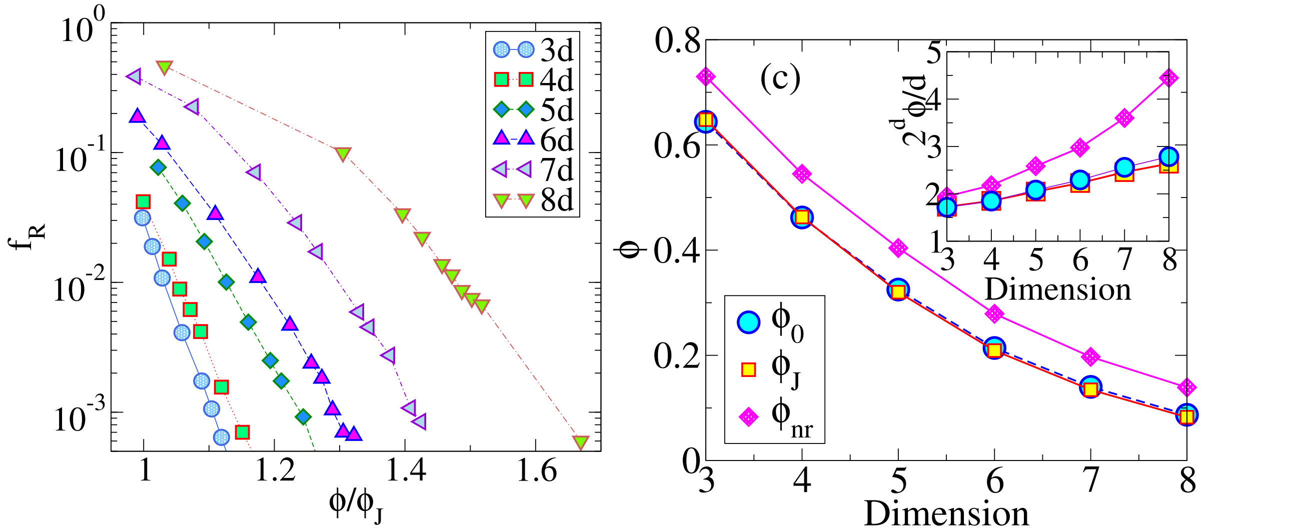


FIG. S10. Left: Fraction of rattlers as a function of density (scaled with the jamming density, $\phi_J$) for $3-8$ spatial dimensions. Right: $\phi_{nr}$ is plotted along with $\phi_J$ and $\phi_0$ as a function of spatial dimension. Inset: Scaled densities $2^d\phi/d$ shown as a function of spatial dimension.

---


[1] N Lačević, Francis W Starr, TB Schrøder, and SC Glotzer, "Spatially heterogeneous dynamics investigated via a time-dependent four-point density correlation function," The Journal of chemical physics **119**, 7372–7387 (2003).

[2] Ludovic Berthier and Thomas A Witten, "Compressing nearly hard sphere fluids increases glass fragility," EPL (Europhysics Letters) **86**, 10001 (2009).

[3] John A Barker and Douglas Henderson, "Perturbation theory and equation of state for fluids. ii. a successful theory of liquids," The Journal of chemical physics **47**, 4714–4721 (1967).

[4] Moumita Maiti and Michael Schmiedeberg, "Temperature dependence of the transition packing fraction of thermal jamming in a harmonic soft sphere system," Journal of Physics: Condensed Matter **31**, 165101 (2019).

[5] Matthieu Mangeat and Francesco Zamponi, "Quantitative approximation schemes for glasses," Physical Review E **93**, 012609 (2016).

[6] Giovanni Brambilla, Djamel El Masri, Matteo Pierno, Ludovic Berthier, Luca Cipelletti, George Petekidis, and Andrew B Schofield, "Probing the equilibrium dynamics of colloidal hard spheres above the mode-coupling glass transition," Physical review letters **102**, 085703 (2009).

[7] Ludovic Berthier and Thomas A Witten, "Glass transition of dense fluids of hard and compressible spheres," Physical Review E **80**, 021502 (2009).

[8] Patrick Charbonneau, Atsushi Ikeda, Giorgio Parisi, and Francesco Zamponi, "Glass transition and random close packing above three dimensions," Physical review letters **107**, 185702 (2011).

[9] Peter K Morse and Eric I Corwin, "Geometric signatures of jamming in the mechanical vacuum," Physical review letters **112**, 115701 (2014).

[10] Patrick Charbonneau and Peter K Morse, "Memory formation in jammed hard spheres," Physical review letters **126**, 088001 (2021).
